# Supplementary material for: Proactive Multi-Camera Collaboration For 3D Human Pose Estimation
Source: arXiv:2303.03767 source file (2023-03-07)
Supplement: Supplementary file 1 [file appendix.tex]

\subsection{Training Details}
At the training stage, we sample random goals for each human and the built-in navigation system helps to generate collision-free trajectories. Each human also walks at a varying speed. Thus, we can simulate dynamic human crowds that exhibit authentic human-like behaviors. To ensure the generalization across a different number of humans, we train our RL policy with a mixture of environments from $1$ to $6$ humans. Similar to the previous works \cite{tallamraju2020aircaprl, ho20213d}, we train and ablate our method on the control of $2$ UAVs. The learning rate is set to $10^{-4}$ during the training phase. Maximum episode length is 500 steps, discounted factor $\gamma$ is 0.99 and GAE horizon is 25 steps. Each sampling iteration produces a training batch with the size of 1,500 steps, then we perform 50 iterations on every training batch with 4 SGD mini-batch updates for each iteration.

For fair evaluation, we reported all of the mean metrics based on the data of 100 episodes and over environments with 1 to 6 humans (class size is uniformly sampled), approximately 800,000 time-steps of agents' experiences. In all experiments, cameras and humans interact in a 10m-by-10m area.
